# Supplementary material for: Seamlessly Unifying Attributes and Items: Conversational Recommendation for Cold-Start Users
Source: arXiv:2005.12979 source file (2022-10-05)
Supplement: Supplementary file 1 [file appendix.tex]

\section{appendix}

\endinput
